# Supplementary material for: Two Causal Principles for Improving Visual Dialog
Source: arXiv:1911.10496 source file (2025-12-10)
Supplement: Supplementary file 1 [file supp.pdf]

## Supplementary Material

This supplementary material will give further details for the main paper, including A. More basic knowledge of causal graph for a better understanding, B. What the confounder brings to us and why we use *do*, C. Proofs and details which are omitted in the main paper due to space limitation, D. More qualitative examples to testify the effectiveness, E. The whole tables including other metrics.

### A. Basic Knowledge of Causal Graph

#### A.1. Causal Graph

The basic definition of causal graph is introduced in the main paper. Here, we introduce more details. The most naive configuration is  $X \rightarrow Y$ , which denotes  $X$  causes  $Y$ , or  $Y$  listens to  $X$ . This directed path from  $X$  to  $Y$  is called causal path, which denotes  $X$ 's causal effect on  $Y$ . In the real world, what we want to know is the causal effect among variables, not just co-occurrence.

For easy to understand the theories we will introduce later, we start from the simple causal graph configurations. There are three basic configurations in causal graph. 1) **Chain**—one arrow directed into and one arrow directed out of the middle variable—is shown in Figure 1(a). 2) **Fork**—two arrows emanating from the middle variable—is shown in Figure 1(b). 3) **Collider**—the middle variable receiving arrows from two other nodes—is like the configuration  $X \rightarrow Z \leftarrow Y$ , which is not shown in the picture because we will not use it.

#### A.2. Conditional independence

We introduce the dependency between variables in causal graph in this section. Using **Chain** shown in Figure 1(a) as an example, it is obvious that:

**$X$  and  $Z$  are dependent**

*i.e.*, for some  $x, z$ ,  $P(Z = z|X = x) \neq P(Z = z)$ ,

**$Z$  and  $Y$  are dependent**

*i.e.*, for some  $z, y$ ,  $P(Y = y|Z = z) \neq P(Y = y)$ ,

These two points are valid because according to the definition of causal graph, child node (*i.e.*,  $Z$  or  $Y$ ) listens to its parent node (*i.e.*,  $X$  or  $Z$ ).

**$X$  and  $Y$  are likely dependent**

*i.e.*, for some  $x, y$ ,  $P(Y = y|X = x) \neq P(Y = y)$ ,

**$X$  and  $Y$  are independent, conditional on  $Z$**

*i.e.*, for all  $x, y, z$ ,  $P(Y = y|Z = z, X = x) = P(Y = y|Z = z)$ .

Here, we're only comparing cases where the value of  $Z$  is constant. Since  $Z$  does not change, the values of  $X$  and  $Y$  do not change in accordance with it. Therefore, any additional changes in the values of  $X$  and  $Y$  must be independent of each other. For example, we use  $X, Z, Y$  to represent three events "there is fire", "there is smoke" and

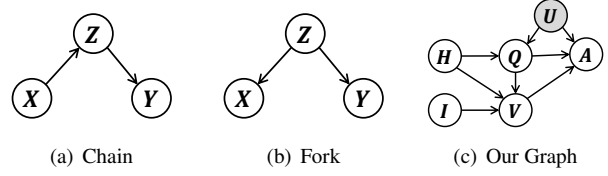

Figure 1. Examples of some causal graph configurations and our graph of visual dialog

"smoke detector is on" respectively. If  $Z$  is always equal to 1 (*e.g.*, "there is smoke" is always true), we will find that  $X$  will not influence  $Y$ , because whether "fire" is on, the event "smoke detector is on" is always true. Therefore,  $X$  and  $Y$  are independent conditional on  $Z$ . In the **Fork** shown in Figure 1(b), the conditional independence relationship among  $X, Y$  and  $Z$  is also satisfied (*i.e.*,  $X$  and  $Y$  are independent, conditional on  $Z$ ).

### B. Causal Effect, Confounder and *do*

In this section, we will give a systematical analysis of the influence of confounder, why we need *do* and how to calculate it. First, we need to give explanation of causal effect. Note that, in the following parts, capital letter denotes variable and lowercase denotes value.

#### B.1. Causal Effect

In the naive causal graph  $X \rightarrow Y$ , the effect of  $X$  on  $Y$  should be  $P(Y|X) - P(Y)$ . For the prior  $P(Y)$ , it is a constant. Therefore, for convenience, in this paper, we sometimes use  $P(Y|X)$  to represent the effect of  $X$  on  $Y$ . Note that there is only one path from  $X$  to  $Y$ , that means the effect from  $X$  on  $Y$  can only pass through the causal path. So,  $P(Y|X)$  is the causal effect. However, in the real world, things are not easy like this.

#### B.2. Confounder

The definition of confounder is introduced in Section 4 in the main paper. Use the **Fork** as an example, by the definition, we know that in Figure 1(b),  $Z$  is the confounder for  $X$  and  $Y$ . In this graph,  $X$  do not have causal effect on  $Y$  because if we only change  $X$  and keep  $Z$ ,  $Y$  will not change (*i.e.*, the causal effect of  $X$  on  $Y$  is 0). When we calculate the causal effect of  $X$  on  $Y$  in this graph, we find that we cannot use  $P(Y|X)$ . That is because the result of  $P(Y|X) - P(Y)$  is not always zero as we mentioned in the Section 4.2 in the main paper. In conclusion, confounder makes us cannot use  $P(Y|X)$  to represent the causal effect, and we need new notations to represent it.

#### B.3. *do*

In the book [6], they introduce a new notation  $P(Y|do(X = x))$ , which can be used to represent the

causal effect of  $X$  on  $Y$ . In this section, we will introduce why it can represent the causal effect and how to calculate it. Note that we will use  $do(X)$  to represent  $do(X = x)$  for concision in the following sections.

**do-operator** As we mentioned in the main paper,  $do$  is a type of intervention, which means that we assign a value to the variable instead of that its parent nodes cause it. For example, in Figure 1(b),  $do(X)$  is that we set variable  $X$  as value  $x$  ignoring its caused function (*i.e.*, arrow  $X \leftarrow Z$ ). Therefore, when we  $do$  a variable, we cut off all the arrows ending to the variable, because its parents do not cause it any more. When we calculate  $P(Y|do(X))$ , no confounder will simultaneously cause  $X$  and  $Y$  because we cut off all the incoming arrows for  $X$ , which ensures our results are causal effect. We will give an example in Section B.4 to testify the statement.

Now, although we have a notation for causal effect, we cannot calculate it by existing methods. We need tool to derive probability formula from  $do$  formula. That is  $do$ -calculus.

**do-calculus** Three rules of  $do$ -calculus are given in [6] to help us derive probability formula.

**Rule 1.** When we observe a variable  $X$  that is irrelevant to  $Y$  (possibly conditional on other variables  $Z$ , like the example “Chain” in Figure 1(a)), then the probability distribution of  $Y$  will not change:

$$P(Y|z, X) = P(Y|z). \quad (1)$$

**Rule 2.** If a set  $Z$  of variables blocks all back-door paths from  $X$  to  $Y$ , then conditional on  $Z$ , like the example “Fork” in Figure 1(b),  $do(X)$  is equivalent to  $see(x)$ :

$$P(Y|do(X), z) = P(Y|X, z). \quad (2)$$

**Rule 3.** We can remove  $do(X)$  from  $P(Y|do(X))$  in any case where there are no causal paths from  $X$  to  $Y$ :

$$P(Y|do(X)) = P(Y). \quad (3)$$

#### B.4. Revisit the Fork

Now, we have  $do$ -operator to represent causal effect and  $do$ -calculus to calculate it. Let us revisit the problem bring by confounder in Section B.2. In Figure 1(b),  $P(Y|do(X))$  can be further written as:

$$\begin{aligned} P(Y|do(X)) &= \sum_z P(Y|do(X), z)P(z|do(X)) \\ &= \sum_z P(Y|z)P(z|do(X)) \\ &= \sum_z P(Y|z)P(z) \\ &= P(Y) \end{aligned} \quad (4)$$

The first line uses Bayes rules, the second one and third one use **Rule 3**. As a result,  $P(Y|do(X)) - P(Y)$  is equal to

0, which accords with our inference for the causal effect of  $X$  on  $Y$  in Section B.2. That also means we can use  $P(Y|do(X))$  to calculate causal effect.

In conclusion, confounder makes us cannot use  $P(Y|X)$  to represent the causal effect, and we obtain a new mathematical notation  $P(Y|do(X))$  to denote it. For calculating  $do$  formula, we need  $do$ -calculus to derive probability formula from it, and the probability formula can be further calculated by observational data. That is the whole story of confounder and  $do$ .

## C. Proofs and Details

### C.1. Proofs of Equation 1

For convenience, we draw our graph in Figure 1(c) and write down the equation again, and add one intermediate step for the formula derivation:

$$\begin{aligned} P(A|do(Q, H, I)) &= \sum_u P(A|do(Q, H, I), u)P(u|do(Q, H, I)) \\ &= \sum_u P(A|do(Q, H, I), u)P(u|do(H)) \\ &= \sum_u P(A|do(Q), H, I, u)P(u|H) \\ &= \sum_u P(A|Q, H, I, u)P(u|H). \end{aligned} \quad (5)$$

According to the rules of  $do$ -calculus introduced in Section B.3, we can derive the following proofs: The first step is according to the Bayes rules. The second one is due to  $Q, I$  do not have a causal path to  $U$  and **Rule 3**. Then, the third step is because  $H, I$  do not have a backdoor to  $A$  and **Rule 2**. As for the last step, although  $Q$  has two backdoors to  $A$  (*i.e.*,  $Q \leftarrow H \rightarrow U \rightarrow A$  and  $Q \leftarrow U \rightarrow A$ ), according to **Rule 2**, when we control  $U$ , all of the backdoors are blocked. As a result, the last transformation is valid.

### C.2. Details of Loss Functions

Following the Equation 4 given in Section 5.2, we give three loss functions:

**Weighted Softmax Loss ( $R_1$ ).**

$$R_1 = \sum_i \log(\text{softmax}(p_i)) \cdot s_i, \quad (6)$$

where  $p_i$  is the logit of candidate  $a_i$ , and  $s_i$  is the corresponding normalized relevance score.

**Binary Sigmoid Loss ( $R_2$ ).**

$$R_2 = \sum_i [\log(\sigma(p_i)) \cdot s_i + \log(\sigma(1 - p_i)) \cdot (1 - s_i)], \quad (7)$$

where  $\sigma$  is the sigmoid function,  $p_i$  is the logit of candidate  $a_i$ , and  $s_i$  is the corresponding normalized relevance score.

**Generalized Ranking Loss ( $R_3$ ).**

$$R_3 = \sum_i \log \frac{\exp(p_i)}{\exp(p_i) + \sum_{j \in G} \exp(p_j)} \cdot s_i, \quad (8)$$

where  $p_i$  is the logit of candidate  $a_i$ ,  $G$  is a group of candidates that has a lower relevance score than  $a_i$ .  $s_i$  is normalized characteristic score (*i.e.*, equals to 0 for  $a_i$  with relevance score 0 and equals to 1 for  $a_i$  with positive relevance score). Note that this function is reorganized from ListNet [2].

### C.3. Proofs of Formula 6

By [8], we can use NWGM [ $\text{softmax}(f_s(e_c, u, m))$ ] (*i.e.*, normalized weighted geometric mean) to approximate  $\mathbb{E}_{[u|H]}[\text{softmax}(f_s(e_c, u, m))]$ . If the probability of  $u$  (*i.e.*, a sample from  $U$ ) is  $P(u_i|H)$ , and  $\text{softmax}(f_s(e_c, u, m)) \propto \exp(f_s(e_c, u, m))$ . We use  $n_{c,i}$  to denote  $f_s(e_c, u, m)$ .  $\mathbb{E}_{[U|H]}[\text{softmax}(f_s(e_c, u, m))]$  can be written as:

$$\begin{aligned} & \mathbb{E}_{[u|H]}[\text{softmax}(f_s(e_c, u, m))] \\ & \approx \text{NWGM}[\text{softmax}(f_s(e_c, u, m))] \\ & = \frac{\prod_i \exp(n_{c,i})^{P(u_i|H)}}{\sum_j \prod_i \exp(n_{j,i})^{P(u_i|H)}} \\ & = \frac{\exp(\mathbb{E}_{[u|H]}[n_{c,i}])}{\sum_j \exp(\mathbb{E}_{[u|H]}[n_{j,i}])}, \end{aligned} \quad (9)$$

where  $j$  is the index of all the candidates. If  $f_s(\cdot)$  is a linear layer, the equation can be further written as:

$$\mathbb{E}_{[u|H]}[\text{softmax}(f_s(e_c, u, m))] \approx \text{softmax}(\mathbb{E}_{[u|H]}[f_s(e_c, u, m)]). \quad (10)$$

### C.4. Details of Principle Implementation

**Details of Enhanced LF[3].** After obtaining the vision and language feature  $\mathcal{H}, \mathcal{Q}, \mathcal{I}$ , we did the further operations (We use the notation *Att* to denote attention operation introduced in main paper): 1) History feature refine:  $\tilde{h} = \text{Att}(\mathcal{H}, q_t)$ , where last term of  $\mathcal{Q}$  (*i.e.*,  $q_t$ ) is guidance. 2) Question and caption feature refine:  $\tilde{q} = \text{Att}(\mathcal{Q}, c_t)$ ,  $\tilde{c} = \text{Att}(\mathcal{C}, q_t)$ . 3) Vision feature refine:  $\tilde{v} = \text{Att}(\mathcal{V}, \{\tilde{q}, \tilde{c}\})$ . 4) Second step of vision feature refine:  $\tilde{v}' = \text{Att}(\tilde{v}, g_v([\tilde{h}; \tilde{q}]))$ , where  $g_v$  is a fully connected layer followed by a Softmax function to generate weights for refining visual attention. 5) Feature fusion:  $e = g_f([\tilde{v}'; \tilde{q}])$ , where  $g_f$  is a multi-head fully connected layer. More details can be found in Table 1.

**Details of P2.** For question type of P2, we manually defined 55 types of questions and then counted the occurrence of ground truth answers under these question types. We set answer candidates with occurrence greater than 5 as preferred answers and annotated their score as 1 under the corresponding question type. At training time, we pre-trained model by original methods for 5 epochs, and gave answer candidates normalized relevance score we counted from question type for every round of each dialog. Then we used the normalized QT-relevance score to further train our

| Index | Input                                 | Operation      | Output                            |
|-------|---------------------------------------|----------------|-----------------------------------|
| (1)   | H (word) (rnd $\times 40$ )           | embed and LSTM | $\mathcal{H}$ (rnd $\times 512$ ) |
| (2)   | C (word) ( $1 \times 20$ )            | embed and LSTM | $\mathcal{C}$ ( $20 \times 512$ ) |
| (3)   | Q (word) ( $1 \times 20$ )            | embed and LSTM | $\mathcal{Q}$ ( $20 \times 512$ ) |
| (4)   | $(\mathcal{H}, q_t)$                  | Attention      | $\tilde{h}$ ( $1 \times 512$ )    |
| (5)   | $(\mathcal{C}, q_t)$                  | Attention      | $\tilde{c}$ ( $1 \times 512$ )    |
| (6)   | $(\mathcal{Q}, c_t)$                  | Attention      | $\tilde{q}$ ( $1 \times 512$ )    |
| (7)   | $(\mathcal{I}, \tilde{q}, \tilde{c})$ | Attention      | $\tilde{v}$ ( $2 \times 2048$ )   |
| (8)   | $(\tilde{v}, [\tilde{h}; \tilde{q}])$ | Attention      | $\tilde{v}'$ ( $1 \times 2048$ )  |
| (9)   | $(\tilde{v}', \tilde{q})$             | Concatenate    | $e$ ( $1 \times 2560$ )           |

Table 1. The details of Enhanced LF Encoder, where rnd is the current number round of history, C is image caption,  $\mathcal{I}$  is the image feature offered by the official with the dimension  $36 \times 2048$  and  $e$  is the output of encoder.

model by  $R_2$ . For Answer Score Sampling, we pre-trained the model for 5 epochs, and then further trained the models by dense annotations with our loss functions. As for the dictionary, we set a  $100 \times 512$  dictionary  $D_u$  to explore the latent representation of  $U$ . We pre-trained the dictionary by one-hot ground truth answer, and then trained the dictionary by  $R_3$  loss with the dense annotations. Then we fused the prediction of the dictionary and the prediction of pre-trained models by  $\text{logit}_i + w \cdot d_i$ , where  $\text{logit}_i$  is the prediction of original models,  $d_i$  is the prediction of the dictionary, and  $w$  is a manually set weight which we set as 0.1. Finally, we further trained the whole model by  $R_3$ .

### C.5. Further Discussion for Metrics

Besides NDCG, there are many other metrics like MRR (*i.e.*, Mean Reciprocal Rank) and R@k (*i.e.*, Recall@k). We ignore these metrics in the main paper is because we think NDCG is better than them to evaluate VisDial task. The reasons are two-fold, 1) The ground-truth for MRR and other metrics is the true answer from a user, whose answer preference (*e.g.*, length) will be consistent in the whole 10-round dialog. Thus, if the user prefers longer answers such as “Yes, I can see a dog”, then a short “Yes” will be unreasonably penalized. We argue that this may be one of the reasons why traditional models with history shortcut have higher MRR, due to the bias illustrated in Figure 2(a) in the main paper. Therefore, if a model has higher MRR, *e.g.*, “Yes, I can see a dog” is scored high, then it must force “Yes” to be low, leading to lower NDCG. That means other metrics (like MRR) have conflicts to NDCG. 2) As we mentioned in Section 1, the answer for VisDial is interactive but VQA has only 1 chance, thus, soft-answer score (NDCG) encourages the interaction better than 1-hot accuracy (MRR) for VisDial task. Last, Note that NDCG is recommended by VisDial organizer—A. Das—who announced in VisDial Workshop 2018 and 2019 that it is the only metric to select winners. As a result, we choose NDCG as only metric and ignore other metrics in the main paper, but for the completeness of the paper, we still give the results on other metrics in Section E.

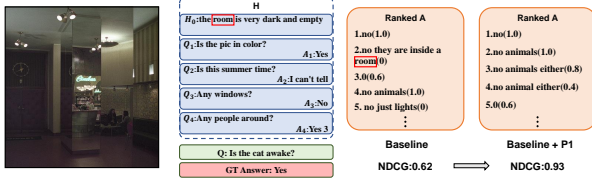

(a) Matching word “room”

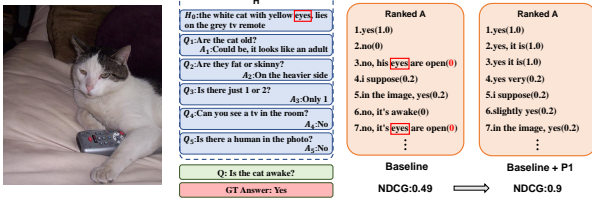

(b) Matching word “eyes”

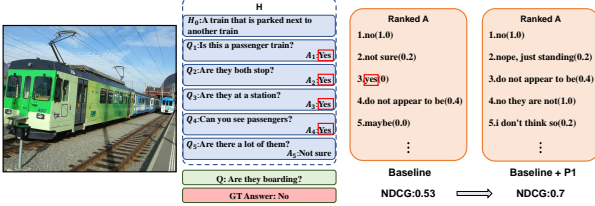

(c) Matching word “yes”

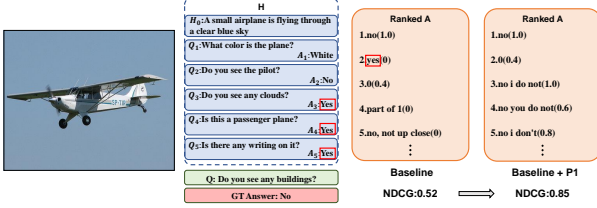

(d) Matching word “yes”

Figure 2. Word Matching

## D. More Qualitative Examples

In this section, we will give more examples of the advantages of our principles mentioned in Section 6, including two types of history bias elimination for P1 shown in Figure 2(a) to Figure 2(d), and better ranking for P2 shown in Figure 3(a) and Figure 3(b).

## E. The Whole Tables

In this section, we will give the whole tables of our experiments, especially results on other metrics omitted in the main paper. These ignored metrics are: 1) mean rank of one-hot ground truth answer (*i.e.*, human response) (**Mean**), 2) recall@k (**R@k**), which is the existence of the human response in the ranked top-k candidates, 3) mean reciprocal

|       | P2         | NDCG(%)      | MRR(%) | R@1(%) | R@5(%) | R@10(%) | Mean |
|-------|------------|--------------|--------|--------|--------|---------|------|
| LF    | baseline   | 57.12        | 64.33  | 50.46  | 81.41  | 90.15   | 4.03 |
|       | QT         | 58.97        | 64.42  | 50.70  | 81.40  | 89.93   | 4.13 |
|       | S( $R_0$ ) | 67.82        | 51.82  | 40.66  | 63.31  | 75.86   | 8.21 |
|       | S( $R_1$ ) | 71.27        | 51.40  | 38.30  | 65.54  | 78.78   | 7.09 |
|       | S( $R_2$ ) | 72.04        | 50.84  | 38.65  | 63.54  | 77.76   | 7.26 |
|       | S( $R_3$ ) | 72.36        | 50.38  | 37.13  | 64.22  | 78.09   | 7.13 |
| LF+P1 | D          | 72.65        | 50.18  | 37.11  | 64.50  | 78.59   | 7.08 |
|       | baseline   | 61.88        | 61.46  | 47.46  | 78.63  | 88.12   | 4.58 |
|       | QT         | 62.87        | 62.09  | 48.13  | 79.40  | 88.79   | 4.47 |
|       | S( $R_0$ ) | 69.47        | 50.54  | 39.71  | 61.41  | 74.55   | 8.72 |
|       | S( $R_1$ ) | 72.16        | 51.20  | 38.56  | 64.78  | 77.96   | 7.46 |
|       | S( $R_2$ ) | 72.85        | 50.93  | 38.88  | 63.41  | 77.66   | 7.35 |
|       | S( $R_3$ ) | 73.42        | 50.53  | 38.41  | 63.12  | 77.54   | 7.40 |
|       | D          | <b>73.63</b> | 50.56  | 37.99  | 63.98  | 77.95   | 7.26 |

Table 2. The whole table of comparison for the experiments of applying our principles on the validation set of VisDial v1.0. LF is the enhanced version as we mentioned. QT, S and D denote question type, answer score sampling, and hidden dictionary learning, respectively.  $R_0$ ,  $R_1$ ,  $R_2$ ,  $R_3$  denote regressive loss, weighted softmax loss, binary sigmoid loss, and generalized ranking loss, respectively.

| Model     | P        | NDCG(%)      | MRR(%) | R@1(%) | R@5(%) | R@10(%) | Mean |
|-----------|----------|--------------|--------|--------|--------|---------|------|
| LF [3]    | baseline | 57.12        | 64.33  | 50.46  | 81.41  | 90.15   | 4.03 |
|           | +P1      | 61.88        | 61.46  | 47.46  | 78.63  | 88.12   | 4.58 |
|           | +P2      | 72.65        | 50.18  | 37.11  | 64.50  | 78.59   | 7.08 |
|           | +P1+P2   | <b>73.63</b> | 50.56  | 37.99  | 63.98  | 77.95   | 7.26 |
| HCIAE [4] | baseline | 56.98        | 64.13  | 50.31  | 81.42  | 90.18   | 4.09 |
|           | +P1      | 60.12        | 61.00  | 46.66  | 78.74  | 88.34   | 4.61 |
|           | +P2      | 71.50        | 46.96  | 32.43  | 63.47  | 78.43   | 7.28 |
|           | +P1+P2   | 71.99        | 46.83  | 33.20  | 61.64  | 76.53   | 7.67 |
| CoAtt [7] | baseline | 56.46        | 63.81  | 49.77  | 81.20  | 90.19   | 4.13 |
|           | +P1      | 60.27        | 60.97  | 46.83  | 78.29  | 87.86   | 4.66 |
|           | +P2      | 71.41        | 47.32  | 33.35  | 63.51  | 77.26   | 7.56 |
|           | +P1+P2   | 71.87        | 46.41  | 32.79  | 61.27  | 76.37   | 7.87 |
| RvA [5]   | baseline | 56.74        | 64.49  | 50.67  | 81.64  | 90.50   | 3.98 |
|           | +P1      | 61.02        | 62.00  | 47.99  | 79.14  | 89.04   | 4.42 |
|           | +P2      | 71.44        | 50.33  | 36.85  | 64.94  | 78.81   | 7.05 |
|           | +P1+P2   | 72.88        | 49.34  | 36.62  | 62.96  | 77.75   | 7.44 |

Table 3. The whole table of ablative studies on different models on VisDial v1.0 validation set. P2 indicates the most effective one (*i.e.*, hidden dictionary learning) shown in Table 2. Note that only applying P2 is implemented by the attempts in Section 5 in main paper with the history shortcut.

rank (**MRR**) of the human response in the returned ranked list. Note that these metrics are not suitable for visual dialog according to our discussion.

## References

- [1] Visual Dialog Challenge 2019 Leaderboard. <https://evalai.cloudcv.org/web/challenges/challenge-page/161/leaderboard/483/>.
- [2] Zhe Cao, Tao Qin, Tie-Yan Liu, Ming-Feng Tsai, and Hang Li. Learning to rank: from pairwise approach to listwise approach. In *Proceedings of the 24th international conference on Machine learning*, pages 129–136. ACM, 2007.
- [3] Abhishek Das, Satwik Kottur, Khushi Gupta, Avi Singh, Deshraj Yadav, José MF Moura, Devi Parikh, and Dhruv Batra. Visual dialog. In *Proceedings of the IEEE Conference on Computer Vision and Pattern Recognition*, pages 326–335, 2017.
- [4] Jiasen Lu, Anitha Kannan, Jianwei Yang, Devi Parikh, and Dhruv Batra. Best of both worlds: Transferring knowledge from discriminative learning to a generative visual dialog

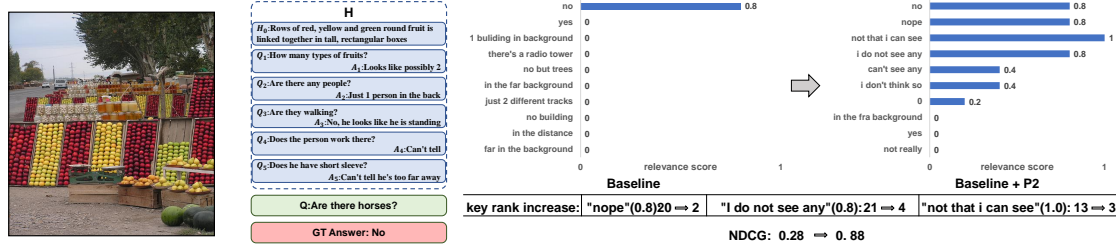

(a) Better ranking for the semantics "no"

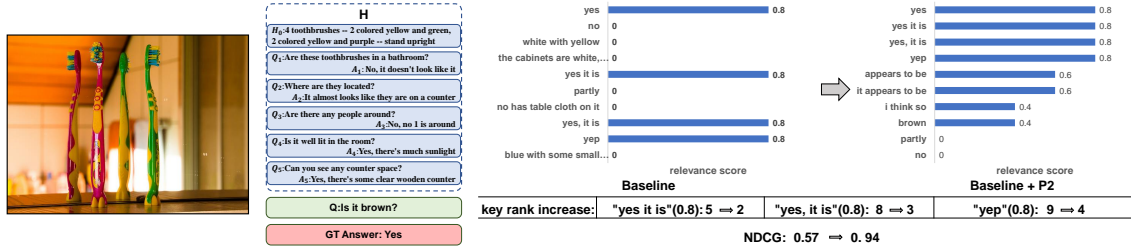

(b) Better ranking for the semantics "yes"

Figure 3. Better Ranking

|             | Model                           | NDCG(%) | MRR(%) | R@1(%) | R@5(%) | R@10(%) | Mean |
|-------------|---------------------------------|---------|--------|--------|--------|---------|------|
| Ours        | P1+P2 (More Ensemble)           | 74.91   | 49.13  | 36.68  | 62.96  | 78.55   | 7.03 |
|             | LF+P1+P2 (Ensemble)             | 74.19   | 46.69  | 32.45  | 62.13  | 77.10   | 7.33 |
|             | LF+P1+P2 (single)               | 71.60   | 48.58  | 35.98  | 62.08  | 77.23   | 7.48 |
|             | RvA+P1+P2 (single)              | 71.28   | 47.71  | 34.80  | 61.53  | 77.10   | 7.63 |
|             | CoAtt+P1+P2 (single)            | 69.81   | 44.83  | 30.83  | 60.65  | 75.73   | 8.08 |
|             | HCIAE+P1+P2 (single)            | 69.66   | 44.03  | 29.85  | 59.50  | 75.98   | 8.10 |
| Leaderboard | VD-BERT(Ensemble)*              | 75.13   | 50.00  | 38.28  | 60.93  | 77.28   | 6.90 |
|             | Tohuku-CV Lab(Ensemble)*        | 74.88   | 52.14  | 38.93  | 66.60  | 80.65   | 6.53 |
|             | MReaL-BDAI*                     | 74.02   | 52.62  | 40.03  | 65.85  | 79.15   | 6.76 |
|             | SFCU(Single)*                   | 72.80   | 45.11  | 32.48  | 57.78  | 74.73   | 7.86 |
|             | FancyTalk(HeteroFM)*            | 72.33   | 54.56  | 42.58  | 67.27  | 80.05   | 6.37 |
|             | Tohuku-CV Lab(Ensemble w/o ft)* | 66.53   | 63.19  | 49.18  | 80.45  | 89.75   | 4.14 |

Table 4. Our results and comparisons to the recent 2019 2nd Visual Dialog Challenge Leaderboard results on the test-std set of VisDial v1.0. Results are reported by the test server, (\*) is taken from [1]. Note that the top five models in the Leaderboard use the dense fine-tune implementation illustrated in Section 5.1.

model. In *Advances in Neural Information Processing Systems*, pages 314–324, 2017.

- [5] Yulei Niu, Hanwang Zhang, Manli Zhang, Jianhong Zhang, Zhiwu Lu, and Ji-Rong Wen. Recursive visual attention in visual dialog. In *Proceedings of the IEEE Conference on Computer Vision and Pattern Recognition*, pages 6679–6688, 2019.
- [6] Judea Pearl and Dana Mackenzie. *THE BOOK OF WHY: THE NEW SCIENCE OF CAUSE AND EFFECT*. Basic Books, 2018.
- [7] Qi Wu, Peng Wang, Chunhua Shen, Ian Reid, and Anton van den Hengel. Are you talking to me? reasoned visual dialog generation through adversarial learning. In *Proceedings of the IEEE Conference on Computer Vision and Pattern Recognition*, pages 6106–6115, 2018.
- [8] Kelvin Xu, Jimmy Ba, Ryan Kiros, Kyunghyun Cho, Aaron Courville, Ruslan Salakhudinov, Rich Zemel, and Yoshua

Bengio. Show, attend and tell: Neural image caption generation with visual attention. In *International conference on machine learning*, pages 2048–2057, 2015.
